# Supplementary material for: Deep Reinforcement Learning of Cell Movement in the Early Stage of C. elegans Embryogenesis
Source: arXiv:1801.04600 source file (2018-03-02)
Supplement: Supplementary file 1 [file supplementary-materials.pdf]

# S1 Model details

## S1.1 Hyperparameters

The hyperparameters for training the neural network in our model is illustrated in Table 1.

| Hyperparameter | Value |
|---|---|
| Tick resolution | 10 secs |
| Batch size | 256 |
| Learning rate $\alpha$ | 0.001 |
| Discount factor $\gamma$ | 0.95 |
| $\epsilon$-greedy factor $\epsilon$ (*Cpaaa intercalation*) | 0.3 to 0.95 (increases by 0.05 every 200 epochs) |
| $\epsilon$-greedy factor $\epsilon$ (*asymmetry rearrangement*) | 0.6 to 0.95 (increases by 0.05 every 50 epochs) |
| Target network replace iteration | 1000 |
| Memory capacity | 8000 |
| Optimizer | Adam($\beta_1 = 0.9$, $\beta_2 = 0.999$) |
| Weight initialization | Isotropic Gaussian ($\mu = 0$, $\sigma = 0.1$) |
| Bias initialization | Constant(0) |

Table 1: Hyperparameter details in the model.

## S1.2 Reward settings

For the *Boundary* rule, a negative reward (penalty) starts to be given when the ratio of the distance between a cell to the eggshell and the radius of that cell is less than 0.8. The penalty grows to 1 (negative reward -1) linearly as the ratio reduces to 0.5. When the ratio is less than 0.5, a terminal condition is triggered (Fig. S1.2(a)). For the *Collision* rule, a negative reward (penalty) starts to be given when the ratio of the distance between two cells and the sum of their radii is less than 0.7. The penalty grows to 1 (negative reward -1) linearly as the ratio reduces to 0.4. When the ratio is less than 0.4, a terminal condition is triggered (Fig. S1.2(b)). For the *Destination* rule, a positive reward starts to be given when the distance between intelligent cell to its target is less than 15. The rewards grows to 14 linearly as the distance reduces to 1. When the distance is less than one, a reward of 20 is given (Fig. S1.2(c)).

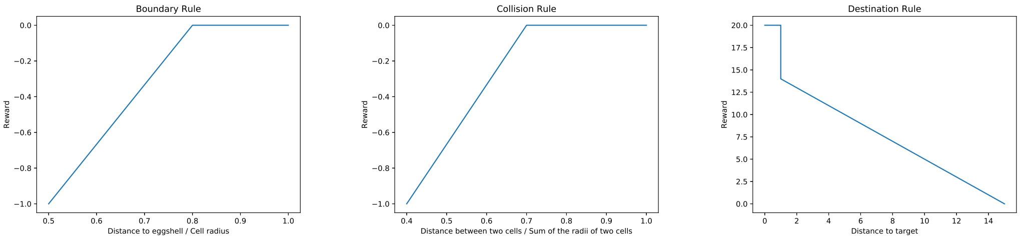


(a) (b) (c)

Figure S1.2: Reward settings in the model.

# S2 Live imaging

The following report strain was used: BV24 ltIs44 [pie-1p-mCherry::PH(PLC1delta1) + unc-119(+)] zuIs178 [(his-72 1kb::HIS-72::GFP) unc-119(+)] V. Nematodes were maintained and handled at 20°C as described [1]. The mounting of embryos was performed as described [2]. In brief, young adult worms were cut using a surgical blade to release their eggs in M9. Embryos in 2-cell stage were mounted on a cover slide in 1$\mu$L M9 containing 50-100 20$\mu$m diameter polystyrene beads (Polysciences Inc.). The M9 drop was covered by a smaller cover slide and sealed with melted Vaseline. Images were taken on a Zeiss AxioObserver Z1 inverted microscope frame with Zeiss 40x objective. 4D Image acquisition was performed in MetaMorph software (Molecular Devices). The resolution of image on XY is 0.254$\mu$m. In total 30 slices were used on Z direction with resolution 1$\mu$m. The image series were acquired from 4-cell stage to 350-cell stage, which roughly takes 240 minutes. Cell lineage [3] was traced by Starrynite II [4] and manually corrected in Acetree [5].

# References


[1] Brenner, S., 1974. The genetics of Caenorhabditis elegans. Genetics, 77(1), pp.71-94.

[2] Bao, Z. and Murray, J.I., 2011. Mounting Caenorhabditis elegans embryos for live imaging of embryogenesis. Cold Spring Harbor Protocols, 2011(9), pp.pdb-prot065599.

[3] Sulston, J.E., Schierenberg, E., White, J.G. and Thomson, J.N., 1983. The embryonic cell lineage of the nematode Caenorhabditis elegans. Developmental biology, 100(1), pp.64-119.

[4] Santella, A., Du, Z. and Bao, Z., 2014. A semi-local neighborhood-based framework for probabilistic cell lineage tracing. BMC bioinformatics, 15(1), p.217.

[5] Boyle, T.J., Bao, Z., Murray, J.I., Araya, C.L. and Waterston, R.H., 2006. AceTree: a tool for visual analysis of Caenorhabditis elegans embryogenesis. BMC bioinformatics, 7(1), p.275.
